# Supplementary material for: A Fast Parameterized Algorithm for Co-Path Set
Source: arXiv:1603.04376 source file (2016-07-27)
Supplement: Supplementary file 1 [file appendix.tex]

This is a test.
